# Supplementary material for: Group testing for overlapping communities
Source: arXiv:2012.02804 source file (2021-03-17)
Supplement: Supplementary file 1 [file AppendixLBP.tex]

\subsection{LBP: message passing rules}

We here describe our loopy belief propagation algorithm (LBP) and update rules for our probabilistic model (II). We use the factor graph framework of \cite{kschischang2001factor} and derive closed-form expressions for the sum-product update rules (see equations (5) and (6) in \cite{kschischang2001factor}).

The LBP algorithm on a factor graph iteratively exchanges messages across the variable and factor nodes. The messages to and from a variable node $\defFamilyVariable_\familyIndex$ or $\defVariable_{\memberIndex}$ are \textit{beliefs} about the variable or distributions (a local estimate of $\Pr(\defFamilyVariable_\familyIndex|\text{observations})$ or $\Pr(\defVariable_{\memberIndex}|\text{observations})$). Since all the random variables are binary, in our case each message would be a 2-dimensional vector $[a,b]$ where $a,b \geq 0$. 
Suppose the result of each test is $y_t$, i.e., $Y_t=y_t$ and we wish to compute the marginals $\Pr(X_e=x|Y_{1}=y_1,Y_{2}=y_2,...,Y_{T}=y_T)$  and  $\Pr(U_v=u|Y_{1}=y_1,Y_{2}=y_2,...,Y_T=y_T)$ for $x,u\in\{0,1\}$. 
The LBP algorithm proceeds as follows:

\begin{figure*}[h!]
	\centering
	\captionsetup{justification=centering}
	\includegraphics[scale=0.48]{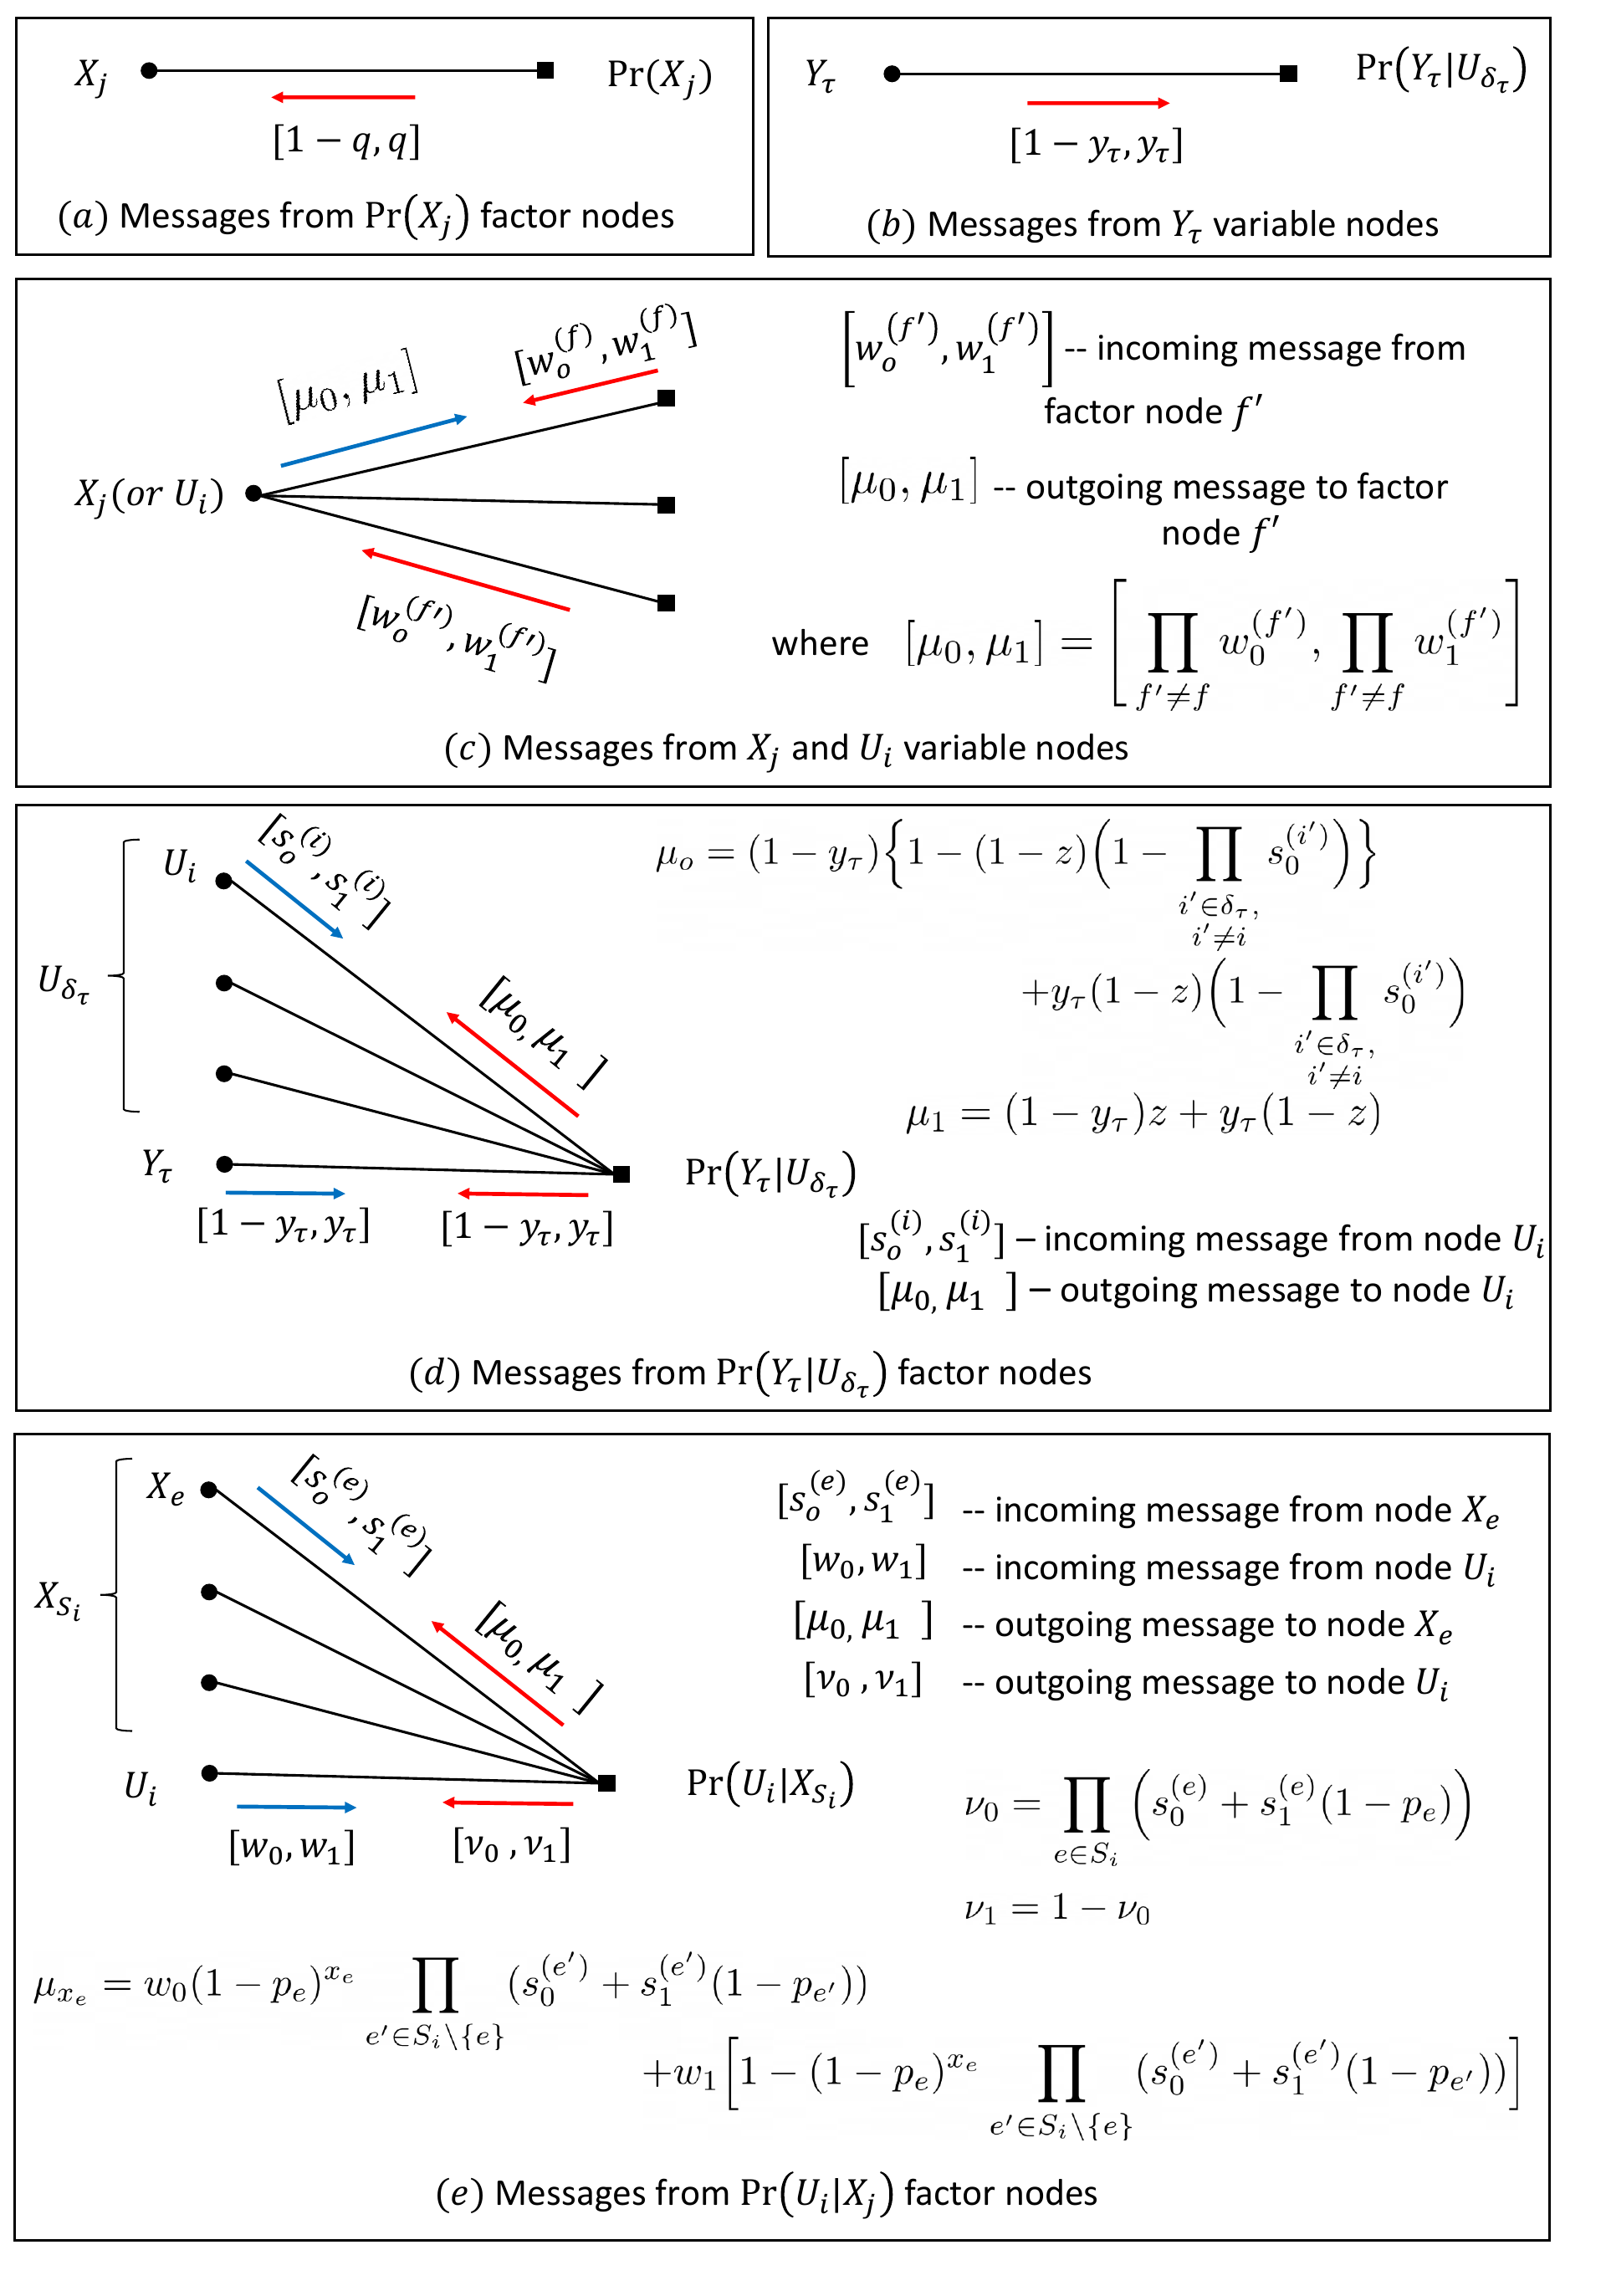}
	\caption{The update rules for the factor and variable node messages.}
	\vspace{-0.2cm}
	\label{fig:messages-appendix}
\end{figure*}

\begin{enumerate}
	\item \textit{Initialization:} The variable nodes $\defFamilyVariable_\familyIndex$ and $\defVariable_{\memberIndex}$ transmit the message $[0.5,0.5]$ on each of their incident edges. Each variable node $Y_\tau$ transmits the message $[1-y_{\tau},y_{\tau}]$, where $y_{\tau}$ is the observed test result, on its incident edge.
	
	\item \textit{Factor node messages:} Each factor node receives the messages from the neighboring variable nodes and computes a new set of messages to send on each incident edge. The rules on how to compute these messages are described next.
	
	\item \textit{Iteration and completion.} The algorithm alternates between steps 2 and 3 above a fixed number of times (in practice 10 or 20 times works well) and computes an estimate of the posterior marginals as follows -- for each variable node $\defFamilyVariable_\familyIndex$ and $\defVariable_{\memberIndex}$, we take the coordinatewise product of the incoming factor messages and normalize to obtain an estimate of $\Pr(\defFamilyVariable_\familyIndex=x|y_1...y_\nTests)$ and $\Pr(\defVariable_{\memberIndex}=\defectValue|y_1...y_\nTests)$ for $x,\defectValue\in\{0,1\}$.
\end{enumerate}

Next we describe the simplified variable and factor node message update rules. We use equations (5) and (6) of \cite{kschischang2001factor} to compute the messages. 
%We omit the intermediate algebraic steps and just state the final update rules:

\textit{Leaf node messages:} At every iteration, the variable node $\testResult_\testIndex$ continually transmits the message $[0,1]$ if $\testResult_\testIndex=1$ and $[1,0]$ if $\testResult_\testIndex=0$ on its incident edge. The factor node $\Pr(\defFamilyVariable_\familyIndex)$ continually transmits $[1-\familyInfectRate,\familyInfectRate]$ on its incident edge; see Fig.~\ref{fig:messages-appendix} (a) and (b).

\textit{Variable node messages:} The other variable nodes $\defFamilyVariable\familyIndex$ and $\defVariable_{\memberIndex}$ use the following rule to transmit messages along the incident edges: for incident each edge $e$, a variable node takes the elementwise product of the messages from every other incident edge $e'$ and transmits this along $e$; see Fig.~\ref{fig:messages-appendix} (c).

\textit{Factor node messages:} For the factor node messages, we calculate closed form expressions for the sum-product update rule (equation (6) in \cite{kschischang2001factor}). The simplified expressions are summarized in Fig.~\ref{fig:messages-appendix} (d) and (e). Next we briefly describe these calculations. 

Firstly, we note that each message represents a probability distribution. One could, without loss of generality, normalize each message before transmission. Therefore, we assume that each message $\mu=[a,b]$ is such that $a+b=1$. Now, the the leaf nodes labeled $\Pr(V_j)$ perennially transmit the prior distribution corresponding to
$V_j$. 

Next, consider the factor node $\Pr(U_i|X_{S_i})$ as shown in Fig.~\ref{fig:messages-appendix} (e). The message sent to $U_i$ is calculated as 
\begin{align*}
\nu_0 &=\sum_{\{x_e\in\{0,1\}:e\in S_i\}} \Pr(U_i=0|X_{S_i}=x_{S_i}) \prod_{e\in S_i} s^{(e)}_{x_e}\\
&=\sum_{\{x_e\in\{0,1\}:e\in S_i\}} \prod_{e\in S_i} (s^{(e)}_{x_e} (1-p_e)^{x_e})\\
&=\prod_{e\in S_i} (s^{(e)}_0 + s^{(e)}_1(1-p_e)).
\end{align*}
Similarly, $\nu_1$ can be computed to be $\nu_1=1-\nu_0$. Now, the message sent to each $X_e$ is 
\begin{align*}
\mu_{x_e} &=\sum_{\substack{u\in{0,1},\\ \{x_{e'}\in\{0,1\}:e'\in S_i\setminus \{e\} \}}} \hspace{-5mm} \Pr(U_i=u|X_{S_i}=x_{S_i}) w_u \prod_{e'\in S_i\setminus \{e\}} s^{(e')}_{x_{e'}}\\
&=\sum_{\substack{\{x_{e'}\in\{0,1\}:e'\in S_i\setminus \{e\} \}}} \Big( \prod_{e'\in S_i\setminus \{e\}} s^{(e')}_{x_{e'}}\Big)\Big (w_0\prod_{e' \in S_i} (1-p_{e'})^{x_{e'}}\\
&+w_1(1-\prod_{e'\in S_i} (1-p_{e'})^{x_{e'}})\Big)\\
&=w_0(1-p_e)^{x_e} \prod_{e'\neq e} (s^{(e')}_0 + s^{(e')}_1(1-p_{e'}))\\
&+ w_1\Big[1- (1-p_e)^{x_e} \prod_{e'\neq e} (s^{(e')}_0 + s^{(e')}_1(1-p_e') \Big ].
\end{align*}

Finally for the factor nodes $\Pr(Y_{\tau}|U_{\delta_{\tau}})$ as shown in Fig.~\ref{fig:messages-appendix} (d), note that the messages to $Y_{\tau}$ play no role since they are never used to recompute the variable messages. The messages to $U_i$ nodes are expressed as 
\begin{align*}
\mu_u &= \sum_{\substack{y\in\{0,1\},\\ \{u_{i'}\in \{0,1\}: i'\in \delta_{\tau}\setminus\{i\}\}}} \Big( \Pr(Y_{\tau}=y|U_{\delta_{\tau}}=u_{\delta_{\tau}})\\ &\hspace{3cm}(1-y_{\tau})^{1-y} y_{\tau}^y \prod_{i'\in \delta_{\tau}\setminus\{i\}\}} s_{u_{i'}}^{(i')} \Big)\\
 &= (1-y_{\tau})\sum_{\substack{\{u_{i'}\in \{0,1\}:\\ i'\in \delta_{\tau}\setminus\{i\}\}}} \Big( \Pr(Y_{\tau}=0|U_{\delta_{\tau}}=u_{\delta_{\tau}}) \\
 &\hspace{4cm} \prod_{i'\in \delta_{\tau}\setminus\{i\}\}} s_{u_{i'}}^{(i')} \Big)\\
  &+ y_{\tau}\sum_{\substack{\{u_{i'}\in \{0,1\}:\\ i'\in \delta_{\tau}\setminus\{i\}\}}} \Big( \Pr(Y_{\tau}=1|U_{\delta_{\tau}}=u_{\delta_{\tau}}) \prod_{i'\in \delta_{\tau}\setminus\{i\}\}} s_{u_{i'}}^{(i')} \Big).
\end{align*}
From our Z-channel model, recall that $\Pr(Y_{\tau}=0|U_{\delta_{\tau}}=u_{\delta_{\tau}}) = 1$ if $u_i=0\ \forall\ i \in \delta_{\tau}$ and $\Pr(Y_{\tau}=0|U_{\delta_{\tau}}=u_{\delta_{\tau}}) = z$ otherwise. Thus we split the summation terms into 2 cases -- one where  $u_{i'}=0$ for all $i'$ and the other its complement. Also combining this with the assumption that the messages are normalized, i.e., $s^{(i)}_0+s^{(i)}_1=1,$ we get 
\begin{align*}
    \sum_{\substack{\{u_{i'}\in \{0,1\}:\\ i'\in \delta_{\tau}\setminus\{i\}\}}} &\Big( \Pr(Y_{\tau}=0|U_{\delta_{\tau}}=u_{\delta_{\tau}}) \prod_{i'\in \delta_{\tau}\setminus\{i\}\}} s_{u_{i'}}^{(i')} \Big)\\
    &= \mathbbm{1}_{u=1}z + \mathbbm{1}_{u=0}\Big\{ 1-(1-z)(1-\prod_{\substack{i'\in\delta_{\tau}\\i'\neq i}} s^{(i')}_0) \Big\},
\end{align*}
and
\begin{align*}
    \sum_{\substack{\{u_{i'}\in \{0,1\}:\\ i'\in \delta_{\tau}\setminus\{i\}\}}} &\Big( \Pr(Y_{\tau}=1|U_{\delta_{\tau}}=u_{\delta_{\tau}}) \prod_{i'\in \delta_{\tau}\setminus\{i\}\}} s_{u_{i'}}^{(i')} \Big)\\
    &= \mathbbm{1}_{u=1}(1-z) + \mathbbm{1}_{u=0}\Big( (1-z)(1-\prod_{\substack{i'\in\delta_{\tau}\\i'\neq i}} s^{(i')}_0) \Big).
\end{align*}
Substituting $u=0$, and $u=1$ we obtain the messages
\begin{align*}
\mu_0 &= (1-y_{\tau})\Big\{ 1-(1-z)(1-\prod_{\substack{i'\in\delta_{\tau}\\i'\neq i}} s^{(i')}_0) \Big\}\\
&+ y_{\tau} (1-z)(1-\prod_{\substack{i'\in\delta_{\tau}\\i'\neq i}} s^{(i')}_0),
\end{align*}
and
\begin{align*}
\mu_1 &= (1-y_{\tau})z+y_{\tau}(1-z).
\end{align*}
For our probabilistic model, the complexity of computing the factor node messages increases only linearly with the factor node degree.
