# Supplementary material for: Group testing for overlapping communities
Source: arXiv:2012.02804 source file (2021-03-17)
Supplement: Supplementary file 2 [file AppendixNoisy.tex]

%============================================
\subsection{Testing with noise}\label{sec:Noisy-Testing}
%============================================
We now compare the two algorithms: (1) two stage algorithm leveraging the community structure but not overlaps; (2) two stage algorithm leveraging the community and overlap structures. 
The only difference lies in the first stage, where for (1) we perform group testing to identify the infected communities using one pooled sample from each community. 

For performance analysis, we consider the special community structure where each member is contained in at most two communities as illustrated in Fig.~\ref{fig-2overlap}. 

Let $\nTests_{c,1},\nTests_{c,2},\nTests_{c,3}$ be the number of tests in the two-stage algorithms for community testing, testing non-infected communities, and testing infected communities for algorithm (1), respectively. 
We use the same number of community tests and tests for $\GroupTestItemSet$ in the two algorithm, 
i.e., $\nTests_{c,1}=\nTests_1$ and $\nTests_{c,2}=\nTests_2$. 
Since algorithm (1) may identify some non-infected overlapped communities as infected, so $\nTests_{c,3}\geq \nTests_{3}$ and thus the total number of tests in (1) may be larger than $\nTests$. 
The expected value of the difference $\nTests_{c,3}-\nTests_{3}$ can be obtained as follows 
\begin{align}
	\mathbb{E}[\nTests_{c,3}-\nTests_{3}]&= (1-\znoiseProb)\nFamilies_o \nMembersSymmetric\cdot \Pr(\text{non-infected community } i \text{ overlap with infected communities})  \\
	&\geq (1-\znoiseProb)\nFamilies_o \nMembersSymmetric\cdot \Pr(j\text{ is infected, } i \text{ is non-infected}| \text{communities } i,j \text{ overlap})  \\
	&=(1-\znoiseProb)\nFamilies_o \nDefFamilies\cdot \frac{{\nFamilies-2 \choose \nDefFamilies-1}}{{\nFamilies \choose \nDefFamilies}}  \\
	&=\frac{(1-\znoiseProb)\nFamilies_o \nMembersSymmetric\nDefFamilies(\nFamilies-\nDefFamilies)}{\nFamilies(\nFamilies-1)},  \label{compare-T3}
\end{align}
where recall that $\nFamilies_o$ is the number of communities that have overlaps with others, 
and the first inequality follows because community $i$ may also have overlaps with other communities. 
We use the following notations. 
\begin{align}
	Q_{c} &= \Pr(FN|\text{community. no overlap}) & Q_{c,1} &= \Pr(FN|\text{Stage 1, community}) \\
	Q_{c,2} &= \Pr(FN|\text{Test } \GroupTestItemSet, \text{ community}) & Q_{c,3} &=\Pr(FN|\text{Test } \IndividualTestItemSet, \text{ community})
\end{align}
We consider the case where $\nDefMembersSymmetric \approx \nMembersSymmetric$, i.e., almost all members of an infected community are infected; we can then choose to label all members in $\IndividualTestItemSet$ as infected. 
In such a case $Q_{c,3} = 0$ and $Q_{3}=0$, at the cost of a slight increase in false positive probability \cite{GroupTesting-community}. 

From the FN probability for group testing in \eqref{FN-prob}, we have 
\begin{align}
	&Q_{c,1}\leq \exp\left[-\frac{2\nTests_1}{\nDefFamilies+N_{1,0}}(\znoiseProb\delta)^2\right], \quad Q_{c,2}\leq \exp\left[-\frac{2\nTests_2}{k_{c,2}}(\znoiseProb\delta)^2\right]\approx \exp\left[-\frac{2\nTests_2}{Q_{c,1}\nDefFamilies\nDefMembersSymmetric}(\znoiseProb\delta)^2\right].  \label{Q-bound-community}
\end{align}
where $N_{1,0}$ is the number of non-infected communities that have overlaps with infected communities, which is equal to $N_{1,0}= \frac{\mathbb{E}[\nTests_{c,3}- \nTests_{3}]} {(1-\znoiseProb)\nMembersSymmetric}$; and $k_{c,2}$ is the expected number of infected members in $\GroupTestItemSet$ which similar to \eqref{k-o2}, can be obtained as $k_{c,2}\approx Q_{c,1}\nDefFamilies\nDefMembersSymmetric$. 

Now we want to compare $Q_o$ against $Q_c$. 
Consider two classes of infected members: (i) infected members included in only one community; (ii) infected members in overlaps. 
\begin{enumerate}[(i)]
	\item For infected members included in only one community, we have 
	\begin{align}
		Q_c&= Q_{c,1}Q_{c,2}+(1-Q_{c,1})Q_{c,3}\approx Q_{c,1}Q_{c,2} \\
		Q_o&= Q_{1}Q_{2}+(1-Q_{1})Q_{3}\approx Q_{1}Q_{2}.
	\end{align}
	From \eqref{Q-bound-overlap} and \eqref{Q-bound-community}, we can see that $Q_{1}<Q_{c,1}$ and $Q_{2}<Q_{c,2}$, which implies that 
	\begin{equation}
		\Pr(FN|\text{overlap})\approx Q_{1}Q_{2}<Q_{c,1}Q_{c,2}.  \label{compare-alg2,3-comb}
	\end{equation}
	More specifically, we have 
	\begin{align}
		\Pr(FN|\text{overlap})&\leq e^{-\frac{2\nTests_1}{\nDefFamilies}(\znoiseProb\delta)^2} e^{-\frac{2\nTests_2}{Q_{1}\nDefFamilies \nDefMembersSymmetric}(\znoiseProb\delta)^2}  \\
		&= \left(e^{-\frac{2\nTests_1}{\nDefFamilies+N_{1,0}}(\znoiseProb\delta)^2}\right) ^{\frac{\nDefFamilies+N_{1,0}}{\nDefFamilies}} \left(e^{-\frac{2\nTests_2}{Q_{c,1}\nDefFamilies \nDefMembersSymmetric}(\znoiseProb\delta)^2}\right)^{\frac{Q_{c,1}}{Q_{1}}}.
	\end{align}
	Now we see that taking overlap structure into account for testing has an exponential gain against without community structure, i.e., achieving a smaller FN probability with a smaller number of tests (c.f. \eqref{compare-T3}). 
	
	\item For infected members in overlaps (assume overlap of communities $i$ and $j$), we have 
	\begin{align}
		\Pr(FN|\text{community})&= Q_{c,1}^2Q_{c,2}+(1-Q_{c,1}^2)Q_{c,3}\approx Q_{c,1}^2Q_{c,2} \\
		\Pr(FN|\text{overlap})&=\Pr(i\text{ or }j \text{ is infected}|\text{overlap infected})\cdot \left(Q_{1}Q_{2}+(1-Q_{1})Q_{3}\right)  \nonumber \\
		&\quad +\Pr(i\text{ and }j \text{ infected}|\text{overlap infected})\cdot \left(Q_{1}^2Q_{2}+(1-Q_{1}^2)Q_{3}\right) \\
		&\stackrel{Q_{3}\approx 0}{\approx} \frac{2(F-\nDefFamilies)}{2F-\nDefFamilies-1}Q_{1}Q_{2}+\frac{\nDefFamilies-1}{2\nFamilies-\nDefFamilies-1}Q_{1}^2Q_{2}    \label{FN-prob-comb-2}\\
		&\stackrel{\text{sparse}}{\approx} Q_{1}Q_{2}, 
	\end{align}
	where \eqref{FN-prob-comb-2} follows from 
	\begin{align}
		\Pr(\text{one of }i,j \text{ is infected}|\text{overlap of } i,j \text{ is infected})&=\frac{2{F-2 \choose \nDefFamilies-1}}{2\cdot{F-2 \choose \nDefFamilies-1}+{F-2 \choose \nDefFamilies-2}} =\frac{2(F-\nDefFamilies)}{2F-\nDefFamilies-1}   \\
		\Pr(\text{both } i,i \text{ are infected}|\text{overlap of } i,j \text{ is infected})&=\frac{{F-2 \choose \nDefFamilies-2}}{2\cdot{F-2 \choose \nDefFamilies-1}+{F-2 \choose \nDefFamilies-2}} =\frac{\nDefFamilies-1}{2F-\nDefFamilies-1}.
	\end{align}
	The comparison of $\Pr(FN|\text{overlap})$ with $Q$ is the same as that in \eqref{compare-overlap-GT}. 
	Now we need to compare $Q_{c,1}^2Q_{c,2}$ and $Q_{1}Q_{2}$. 
	Let $N_{1,0}=\gamma\nDefFamilies$ (c.f. \eqref{Q-bound-community}) for some $\gamma\in\left(0,\frac{\nFamilies-\nDefFamilies}{\nDefFamilies}\right)$. 
	Then we have 
	\begin{align}
		Q_{c,1}^2Q_{c,2}&\leq \left(e^{-\frac{2\nTests_1}{\nDefFamilies+\gamma\nDefFamilies}(\znoiseProb\delta)^2}\right)^2\cdot  \left(e^{-\frac{2\nTests_2}{Q_{c,1}\nDefFamilies\nDefMembersSymmetric}(\znoiseProb\delta)^2}\right)  \\
		&\leq u^{\frac{2}{1+\gamma}}\cdot \left(e^{-\frac{2\nTests_2}{u^{1/(1+\gamma)}\cdot \nDefFamilies \nDefMembersSymmetric}(\znoiseProb\delta)^2}\right)  \\
		&=(uw)\cdot \left(u^{\frac{1-\gamma}{1+\gamma}}w^{u^{\frac{\gamma}{1+\gamma}}}\right)
	\end{align}
	where the second inequality follows by defining $u\triangleq e^{-\frac{2\nTests_1}{\nDefFamilies}(\znoiseProb\delta)^2}<1$, 
	and the first equality follows by defining $w=e^{-\frac{2\nTests_2}{u\nDefFamilies \nDefMembersSymmetric}(\znoiseProb\delta)^2}$. 
	By the definition of $u$ and $w$, we have $Q_{1}Q_{2}\leq uw$. 
	Thus, we need to compare $f(\gamma)\triangleq u^{\frac{1-\gamma}{1+\gamma}}w^{u^{\frac{\gamma}{1+\gamma}}}$ and 1. 
	By taking derivative, we can see that $f(\gamma)$ is increasing in $\gamma$, and thus $f(\gamma)\in\left(uw,\frac{w^u}{u}\right)$. 
	The upper bound $\frac{w^u}{u}\geq w$ is decreasing in $u$ and can be extremely large for small $u$. 
	
	From the above analysis, we have the following observation: for a large $\gamma$ and small $u$ (small $Q_{1}$), we have $f(\gamma)>1$ and then 
	$\Pr(FN|\text{community})>\Pr(FN|\text{overlap})$; for a small $\gamma$ and large $u$, we have $f(\gamma)<1$ and then $\Pr(FN|\text{community})<\Pr(FN|\text{overlap})$. 
	This is reasonable: (i) for a large $\gamma$, there will be more positive community samples ($\gamma\nDefFamilies$ of them come from infected overlaps) if we do not take overlap into account, then so $\Pr(FN|\text{community})$ will be higher; (ii) a small $u$ means small $\Pr(FN|\text{overlap})$. 
	
	We see that taking overlap into account sometimes does not outperform without overlaps, 
	the reason is that for infected overlapped members, the infection is testes more than one time in stage 1 from all the communities that include this member. 
\end{enumerate}
